# Supplementary material for: A Composable Framework for Policy Design, Learning, and Transfer Toward Safe and Efficient Industrial Insertion
Source: arXiv:2203.03017 source file (2022-03-06)
Supplement: Supplementary file 1 [file appendix_A_CTC.tex]

\subsection{Regulation Problem}

Consider a second-order integrator on Cartesian state and velocity $$x_k:=[x, y, z, rx, ry, rz, \dot{x}, \dot{y}, \dot{z}, \dot{rx}, \dot{ry}, \dot{rz}]^\top$$
\begin{equation}
    x_{k+1} = \begin{bmatrix}
    \mathbf{I} & \Delta_t\cdot\mathbf{I} \\ 0 & \mathbf{I}
    \end{bmatrix} x_k + \begin{bmatrix}
    0.5\Delta_t^2\cdot\mathbf{I} \\ \Delta t\cdot \mathbf{I}
    \end{bmatrix} u_k
\end{equation}
that tracks the goal at origin. The run-time cost is $l_k(x_k, u_k)=\frac{1}{2}x_k^\top Qx_k+\frac{1}{2}u_k^\top Ru_k$. The terminal cost is $l_N(x_N)=\frac{1}{2}x_N^\top Sx_N$. There is an input constraint $u_k\in[-b_u, b_u]$, an orientation constraint $[rx, ry, yz]^\top_k=\mathbf{0}$, a velocity constraint $[\dot{x}, \dot{y}, \dot{z}, \dot{rx}, \dot{ry}, \dot{rz}]_k^\top\in[-b_v,b_v]$, and a terminal state constraint $x_N=\mathbf{0}$.

We solve the following optimization problem for the desired Cartesian trajectory of length $N$.

\begin{align}
    \underset{u_{0:N-1}}{\mathbf{min}} &~\sum_{k=0}^{N-1}l_k(x_k, u_k) + l_N(x_N) \label{eq: mpc_regulation}\\
    \mathbf{s.t.} &~x_{k+1} = \begin{bmatrix} \mathbf{I} & \Delta_t\cdot\mathbf{I} \\ 0 & \mathbf{I} \end{bmatrix} x_k + \begin{bmatrix} 0.5\Delta_t^2\cdot\mathbf{I} \\ \Delta t\cdot \mathbf{I} \end{bmatrix} u_k \\
    &~u_k\in[-b_u, b_u]\\
    &~[\dot{x}, \dot{y}, \dot{z}, \dot{rx}, \dot{ry}, \dot{rz}]_k^\top\in[-b_v,b_v]\\
    &~[rx, ry, yz]^\top_k=\mathbf{0}\\
    &~x_N=\mathbf{0}
\end{align}

\subsection{Tracking Static Reference}

At arm state $x^a_k$, tracking a static reference $x^r$ is equivalent to solving \eqref{eq: mpc_regulation} with the zero order segment of $x_k$ equal to the Cartesian error $x^{error}_k = d(x^a_k, x^r)$. $p^{error}=d(p_1, p_0)$ calculates the transformation from $p_0$ to $p_1$ in Cartesian space. The result written in full transformation matrices should satisfy $T(p^{error})T(p_0)=T(p_1)$ since $p^{error}$ represents the transformation from $p_0$ to $p_1$ in world frame (hence the left product).

Solving \eqref{eq: mpc_regulation} yields $U_k$, the Cartesian accelerations. The corresponding error trajectory $X_k=[x_k^\top, x_{k+1}^\top,\dots,x_{k+N}^\top]^\top$ can be calculated by $X_k = \bar{f}+\bar{B}U_k$. Finally, we can apply the zero order parts of $X_k$ in the form of world frame transformation on $x^r$ to retrieve the desired arm state trajectory, that is
\begin{equation}
    T(x^a_{i,state}) = T(x_{i,state})T(x^r),~\forall i\in[k,\dots,k+N]
\end{equation}

We collect the desired Cartesian trajectory as $X^a_k=\{{x^a_k}, {x^a_{k+1}},\dots,{x^a_{k+N}}\}$.

\subsection{Inverse Kinematics}

In this section, we transform the Cartesian trajectory $X^a_k$ to joint state trajectory $$Q^a_k=\{{q^a_k}, {q^a_{k+1}}^,\dots,{q^a_{k+N}}\}.$$ The relationship between the Cartesian pose and joint state can be written as 
\begin{equation}
    x^a_k= \Gamma(q^a_k)
    \label{eq7}
\end{equation}
where $\Gamma$ is the forward kinematics function. Therefore, given Cartesian trajectory, the transformation from Cartesian trajectory to joint state trajectory is equivalent to find a trajectory of joint states satisfying the above highly nonlinear equality constraints. Here we introduce an iterative optimization approach to find joint state trajectory step by step, the optimization problem at time step $k$ is summarized below:
\begin{equation}
\begin{aligned}
& \underset{q^a_t}{\text{min}}
& & J(q^a_t,q^a_{t-1}) = \| q^a_t - q^a_{t-1}\|_Q^2 \\
& \text{s.t.} & &  \Gamma(q^a_t) = x^a_t
\end{aligned}
\label{eq:opt}
\end{equation}

% \subsection*{Iterative Equality Linearization Approximation}
 In this paper we assume $\Gamma$ is a twice continuously differentiable function whose second derivative exists and is continuous. 
To speed up the computation, we propose to iteratively consider the first order approximation of the nonlinear equality constraint until the solution converges.

Suppose the initial joint state is $q^a_0$, the corresponding Cartesian point is located at $x^a_0$. Our target is to find $x^a_1$ that satisfies $\Gamma(q^a_1) = x^a_1$, where $x^a_1$ is the next desired Cartesian point. Suppose the distance between $x^a_1$ and $x^a_0$ is less than a small positive constant. Then we can use first-order linear approximation to represent $x^a_1$ as:
\begin{align}
x^a_1 &= \Gamma(q^a_0) + \nabla\Gamma(q^a_0)\cdot(q^a_1 - q^a_0) + \sigma, \\
	&= x^a_0 + \nabla\Gamma_j(q^a_0)\cdot(q^a_1 - q^a_0) + \sigma, \label{eq5}
\end{align}
where $\sigma$ is an error term, and $\sigma \to 0$ as $\| q^a_1 - q^a_0 \|_2^2 \to 0 $.  Denote $\nabla \Gamma(q)$ as $Jac(q, \theta)$, which is the generalized Jacobian matrix at $x$ with respect to a robot feature vector $\theta$ such as the DH parameters. Now we rewrite \eqref{eq5} as:
\begin{equation}
Jac(q^a_0,\theta)\cdot q^a_1 = Jac(q^a_0,\theta)\cdot q^a_0 + x^a_1 - x^a_0 - \sigma,
\label{iela}
\end{equation}
which is a linearized equality constraint for \eqref{eq7}. Inspired by iLQR, it is reasonable to assume that solving the optimization \eqref{eq:opt} with respect to the iterative approximation of nonlinear equality constraints in \eqref{iela} will lead to converging results. 

\subsection{Sending Joint Trajectory Command}

Given desired Cartesian trajectory $X^a_k$ and joint state trajectory $Q^a_k$, we can directly calculate the desired joint velocities. At time $k$, we have $\dot{q}^a_k=J(q^a_k)^{-1}{x}^a_{k,vel}$ where $J(q)$ is the jacobian at joint state $q$ and $q^a_k$ is measured joint state. Collecting the interpolated joint velocities $\dot{Q}^a_k=\{{\dot{q}^a_k}, {\dot{q}^a_{k+1}},\dots,{\dot{q}^a_{k+N}}\}$, we send it with $Q^a_k$ to the follow joint trajectory controller for execution.
